# Supplementary material for: Reconstructing Roma history from genome-wide data
Source: arXiv:1212.1696 source file (2012-12-07)
Supplement: Supplementary file 1 [file final-supp.pdf]

# Reconstructing Roma history from genome-wide data

<u>Table of Contents</u>

**Note S1 – New *ROLLOFF* Statistic** 2-6
**Note S2 – Simulations for estimating dates of admixture events** 7-9
**Note S3 – Computing corrected IBD sharing distance between Roma and Indian groups** 10
**Note S4 – Simulations for estimating dates of founder events** 11-12

**Figure S1 – ADMIXTURE Analysis of Roma and HapMap3 populations** 13
**Figure S2 – Estimating the proportion of Eurasian and South Asian ancestry in Roma** 14
**Figure S3 – Normalization term from original *ROLLOFF* correlation coefficient formulation** 15
**Figure S4 – *ROLLOFF* Simulation Results: Variable age of mixture** 16
**Figure S5 – *ROLLOFF* Simulation using PCA-based SNP loadings** 17
**Figure S6 – IBD Sharing of Roma with host European populations** 18
**Figure S7 – Bootstrap analysis to compute error in IBD statistics** 19

**Table S1 – Average frequency differentiation ($F_{st}$) for Roma and HapMap populations** 20
**Table S2 – Formal tests of admixture** 21
**Table S3 – Simulations for estimating dates of admixture events: Founder events post admixture model** 22
**Table S4 – Simulations for estimating dates of admixture events: Two gene flow model** 23
**Table S5 – Simulations for estimating dates of founder events** 24

**References** 25

## NOTE S2. Simulations for estimating dates of admixture events

### Simulation 1: To test the effect of founder events post admixture

In order to test the effect of founder events post admixture, we performed simulations using MaCS[3] coalescent simulator. We simulated data for three populations (say, *A*, *B* and *C*). We set the effective population size ($N_e$) for all populations to 12,500 (at all times except during the founder event), mutation and recombination rate to $2 \times 10^{-8}$ and to $1 \times 10^{-8}$ per base pair per generation respectively. *C* can be considered as an admixed population that has 60%/40% ancestry from *A'* and *B'* (admixture time (*t*) was set to 30/ 100 generations before present). *A'* and *A* diverged 120 generations ago, *B'* and *B* diverged 200 generations ago and *A* and *B* diverged 1800 generations ago. At generation *x* ($x < t$), *C* undergoes a severe founder event where the effective population size ($N_e$) reduces to 5 individuals for one generation. At generation ($x+1$), the $N_e$ = 12,500. We simulate data for 5 replicates for each parameter. We performed *ROLLOFF* analysis (using the original and modified statistics) with *C* as the target and *A* and *B* as the reference populations. When we use the original *ROLLOFF* statistic, we observe that the dates are biased downward in cases of founder events post admixture. However, when we use the modified statistics, the bias is removed (Table S3). Details of the bias correction are shown in Note S1. Throughout the manuscript, we use the modified *ROLLOFF* statistic (*R(d)*) unless specified otherwise.

### Simulation 2: To test the accuracy of the modified *ROLLOFF* statistic

We perform simulations using the same simulation framework as in reference [1] to test the accuracy of the estimated dates using the modified *ROLLOFF* statistic. We simulated data for 25 admixed individuals using Europeans (HapMap CEU) and HGDP East Asians (Han) as ancestral populations, where mixture occurred between 10-300 generations ago and European ancestry proportion was set to

20%. These ancestral populations were chosen as $F_{st}$(CEU, Han) = 0.09 is similar to the $F_{st}$ between the ancestral populations of the Roma. Figure S4 shows that we get accurate estimates for the dates of mixture up to 300 generations.

**Simulation 3: To test the effect of using PCA loadings instead of allele frequencies as weights in *ROLLOFF***

In the case of Roma admixture, data from unadmixed South Asian populations is not available and so it is not possible to compute the allele frequencies of SNPs for one ancestral population. However, data from many South Asian populations (which are admixed with ANI and ASI ancestry) are available and can be used for estimating the PCA-based SNP loadings. We simulations described below that mimic this scenario -

We simulated data for 60 admixed individuals using Europeans (HapMap CEU) and HGDP East Asians (Han) as ancestral populations, where mixture occurred 100 generations ago and European ancestry proportion was set to 30% (group 1: $n$ = 20), 50% (group 2: $n$ = 20) and 70% (group 3: $n$ = 20). These three groups of simulated samples can be roughly considered as three South Asian populations. We performed PCA analysis with CEU and Groups 1-3 of simulated samples to estimate the SNP loadings that can be used in *ROLLOFF*.

Next, we simulated data for 54 individuals that can be used as the target in the *ROLLOFF* analysis. These individuals have 80%/20% European and East Asian ancestry respectively (similar to Roma) and the date of mixture is set to 30 ($n$ = 27) and 100 ($n$ = 27) generations before present. We ran modified *ROLLOFF* statistic to estimate the date of mixture in this panel of individuals using the PCA-based loadings computed above. We estimated that the dates of mixture were 33 ± 1 and 99 ± 1 generation for mixture that occurred 30 and 100 generations ago respectively (Figure S5). This shows that we can effectively estimate the date of mixture even in the absence of data from unadmixed ancestral populations, as

long as data from other admixed individuals (involving the relevant ancestral populations) is available.

**Simulation 4: To test the model of two waves of admixture**

In order to obtain an interpretation of the *ROLLOFF* estimated date of mixture when the model assumption of single wave of mixture is incorrect, we ran modified *ROLLOFF* statistic to infer the date of admixture on data simulated under a double admixture scenario. We simulated data using Europeans (HapMap CEU) and HGDP East Asians (Han) as the ancestral populations using the simulation framework described in reference [1]. We simulated double admixture scenarios in which a 50%/50% admixture of CEU and Han occurred at $\lambda_1$ (shown in Table S4), followed by a 60%/40% mixture of that admixed population and CEU at $\lambda_2$ (shown in Table S4). The mixture proportions were chosen so that the final European ancestry proportion is ~80% (similar to Roma). We ran modified *ROLLOFF* with a non-overlapping set of Europeans and Han as the reference population. Table S4 shows that as the interval ($\lambda_2$-$\lambda_1$) between the multiple waves of mixture increases, the estimated dates of mixture reflects the date of the more recent gene flow event.

## NOTE S3. Computing corrected IBD sharing distance between Roma and Indian groups.

To find the source of the Indian ancestry in Roma, we inferred the pairwise IBD sharing distance between Roma and various Indian groups. We observed that the Roma share the highest proportion of IBD sharing with groups from the northwest of India (Figure 3b). We were concerned that high IBD sharing could be an artifact related to the high proportion of ANI ancestry in the North-western Indian groups. Hence, we performed a regression analysis to correct for the effect of the ANI ancestry proportion on IBD sharing distance. The model that provided the best fit was IBD sharing = 0.3558 + 0.8169*ANI ancestry proportion (P-value < 0.05). Each Indian group was considered as a single data point for this analysis. Next, we computed an average corrected IBD sharing measure for each region by regression out the effect of ANI ancestry and computing an average of the residuals for each region in India. Note: For this analysis, we did not include the Eastern Indian populations (Nyasha and Ao Naga) and Andamanese populations (Onge and Great Andamanese) as these populations do not have ANI ancestry.

In order to control for the effect of the sample size on the IBD computation, we performed bootstrap analysis such that for each run, we randomly sampled up to 30 individuals (some groups had < 30 samples) from each of the 8 Indian groups and estimated the IBD sharing statistics between Roma and the Indian groups. We performed a total of 100 runs and obtained the mean and standard error of the IBD statistic (Figure S7). We observed that Roma still share the highest proportion of IBD segments with groups from Northwest of India.

## NOTE S4. Simulations for estimating date of founder event.

We used MaCS[3] coalescent simulator to perform simulations to test the robustness of our allele sharing statistic that we use for estimating the dates of the founder event. We simulated data for two populations (say, *A* and *B*) that diverged 1800 generations ago. We set the effective population size for both populations as $N_e$ = 12,500, mutation rate = $2x10^{-8}$ and recombination rate = $1x10^{-8}$ per base pair per generation respectively. For each simulation, we compute the autocorrelation of allele sharing within *B*, and then subtract the across-population autocorrelation between *A* and *B* to remove the effects of ancestral allele sharing

**Simulation 1: Founder event only**

Pop *B* undergoes a severe founder event *x* generations ago where the effective population size reduces to 5 individuals for one generation. At generation (*x+1*), the population size = $N_e$ again. Table S5 shows that we can accurately estimate the date of the founder event using our statistic.

**Simulation 2: Founder event and admixture**

We simulate data for a more complex demography where *B* is admixed and has 40% ancestry from *A'* which is closely related to *A*. The admixture occurred at time *t* and at time *x* = 10, 30 or 100 generations, *B* undergoes a severe founder event where the effective population size of *B* reduces to 5 individuals for one generation. Table S5 shows that for a recent founder event (10 and 30 generations ago), we accurately estimate the date of the founder event. However, for older founder events (100 generations), we are unable to accurately estimate the date of the founder event, if it occurred pre-admixture. However, this is expected as we are only sampling the admixed population and not the ancestral population that underwent the founder event.

**Simulation 3: No Founder event**

We simulate data for a complex demography where *B* is admixed and has 40% ancestry from *A'* which is closely related to *A*. The admixture occurred either 10, 30, 50 or 70 generations ago. In all cases, we observe that the allele sharing statistic is not associated to distance. We test if the model of a straight line ( $y \sim c$ ) or exponential decay ( $y \sim c + Ae^{-tD}$ ), where *D* = genetic distance and *t* = time of founder event) is a better fit to the output. In all four cases, we fail to reject the null model ( $y \sim c$) (P > 0.05).

**Figure S1. ADMIXTURE Analysis of Roma and HapMap3 populations**. Results for ADMIXTURE analysis for K=2 to K=7. Each vertical line represents an individual colored in proportion to their estimated ancestry within each cluster.

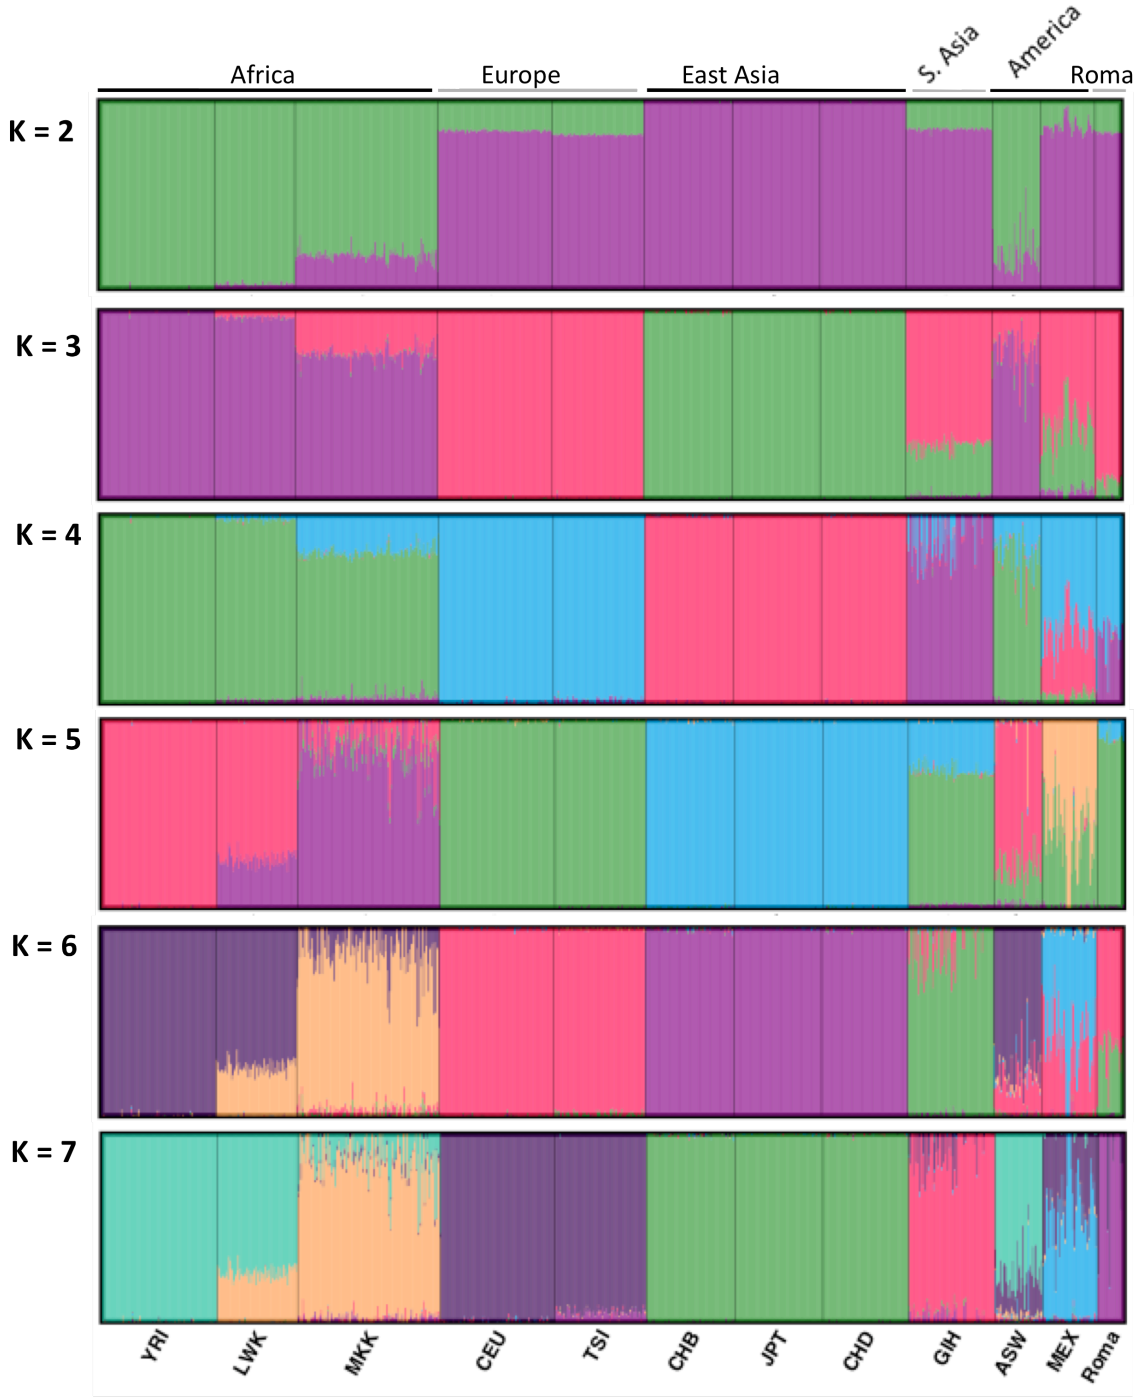

**Figure S2. Estimating the proportion of Eurasian and South Asian ancestry in Roma.** In order to estimate the proportion of West Eurasian ancestry in Roma, we use the phylogenetic tree shown below. The different colored lines show drift that has occurred between the populations connected by the line. The orange line shows the drift between YRI and Adygei (a population from the Caucasus) and the red and green lines shows the drift separating Roma and Onge. *m* denotes the shared drift between Roma and Onge. See methods for details for estimating the West Eurasian ancestry proportion (*p*) in Roma. This figure is adapted from reference [4].

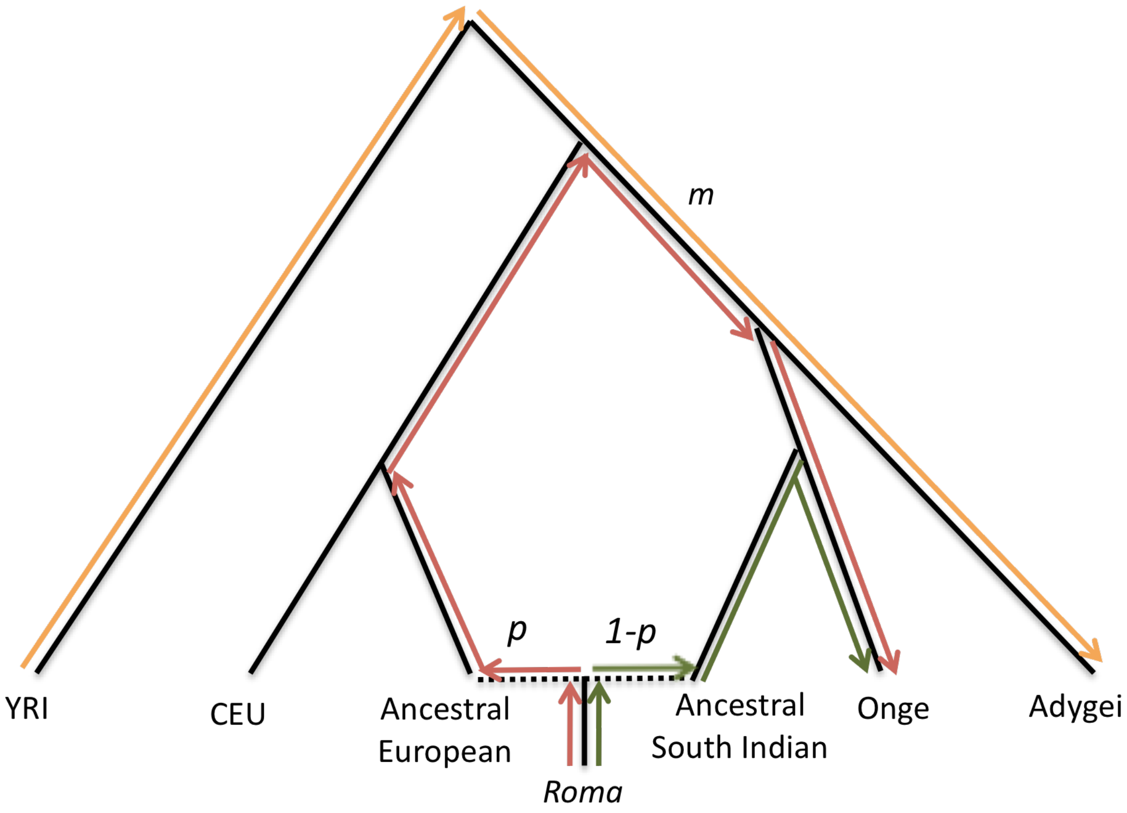

**Figure S3. Normalization term from original *ROLLOFF* correlation coefficient formulation.** We plot the squared normalization term $\sum_{|x-y|\approx d} z(x,y)^2$ as a function of genetic distance *d* between SNPs for the admixture plus bottleneck scenarios described in Table S3, using either the correlation (a) or covariance (b) versions of $z(x,y)$. In the case of no bottleneck, the normalization term is dominated by finite sampling noise and exhibits no dependence on *d*. For the cases of a strong bottleneck post-admixture, however, $\sum_{|x-y|\approx d} z(x,y)^2$ exhibits an exponential decay $Ae^{-2kd} + c$ with rate constant approximately equal to twice the age of the bottleneck (best-fit *k* = 15, 25, 46, 65, 83 (a) and *k* = 12, 20, 41, 60, 78 (b) shown as solid lines).

**(a) Using *z*(*x*,*y*) = correlation(*x*,*y*)**

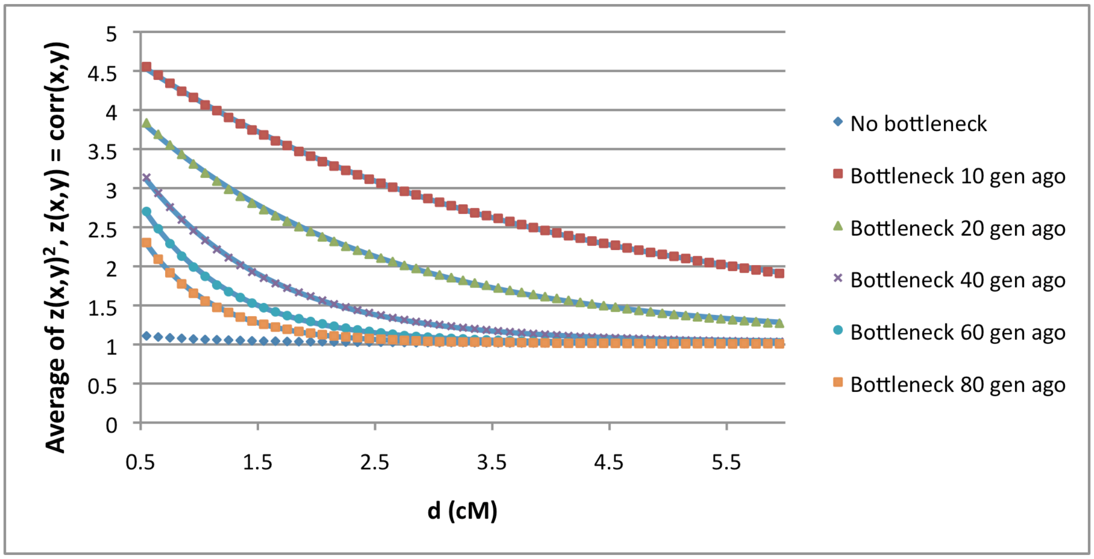


**(b) Using *z*(*x*,*y*) = covariance(*x*,*y*)**

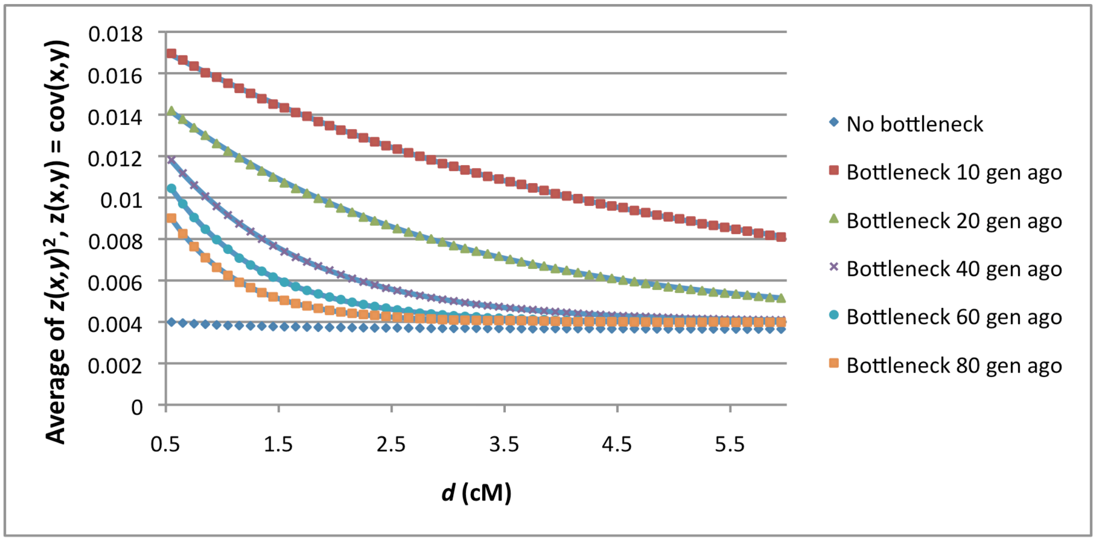

**Figure S4. *ROLLOFF* Simulation Results: Variable age of mixture.** We simulated data for 25 admixed individuals with mixed European and East Asian ancestry where the proportion of European ancestry was set to 20% and set the admixture date between 10-300 generations (as shown below). We ran the modified *ROLLOFF* statistic to estimate the date of mixture using allele frequencies in an independent dataset of French and East Asians. Standard errors were computed using weighted block jackknife as described in the Methods.

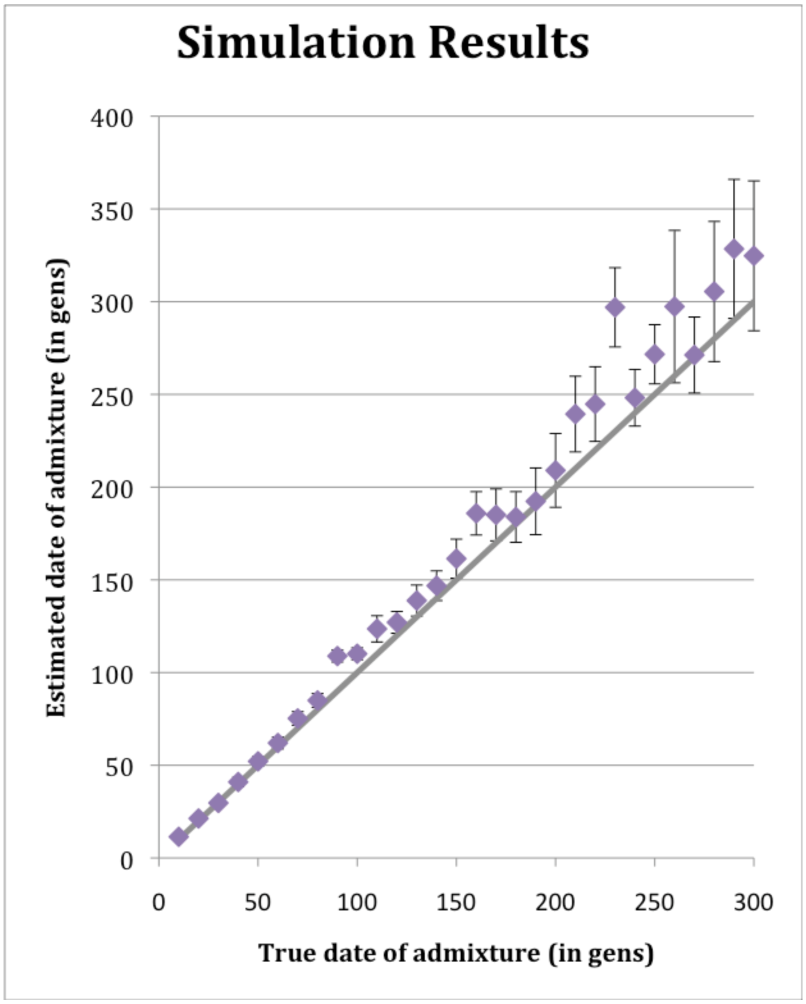

**Figure S5. *ROLLOFF* Simulation using PCA-loadings.** We simulated data for 54 individuals with mixed European and East Asian ancestry where the proportion of European ancestry was set to 80% (similar to Roma) and the mixture occurred 30 generations ago (left panel: $n$ = 27) and 100 generations ago (right panel: $n$ = 27). We ran *ROLLOFF* to estimate the date of mixture in this panel of individuals using the PCA-based loadings computed above. We estimated that the dates of mixture were 33 ± 1 and 99 ± 4 generations (the true dates were 30 and 100).

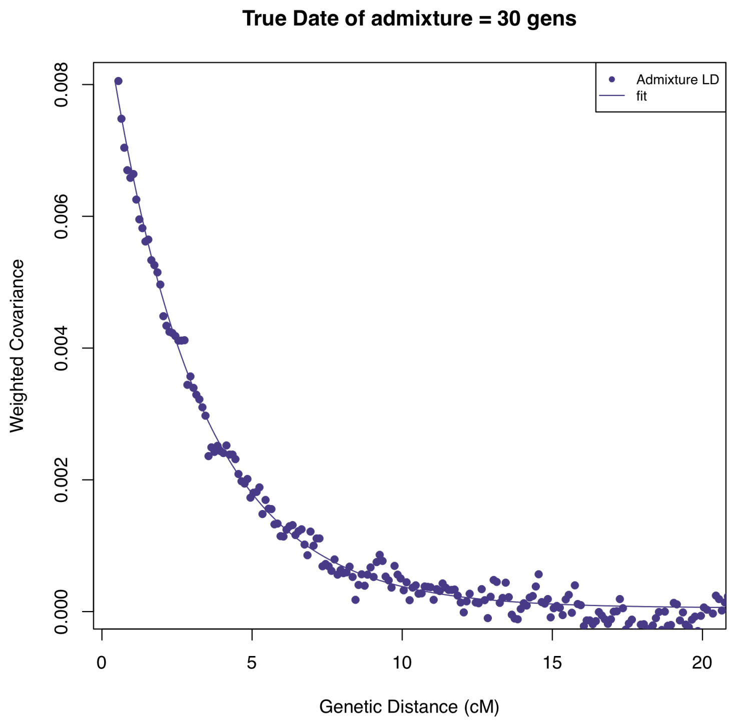


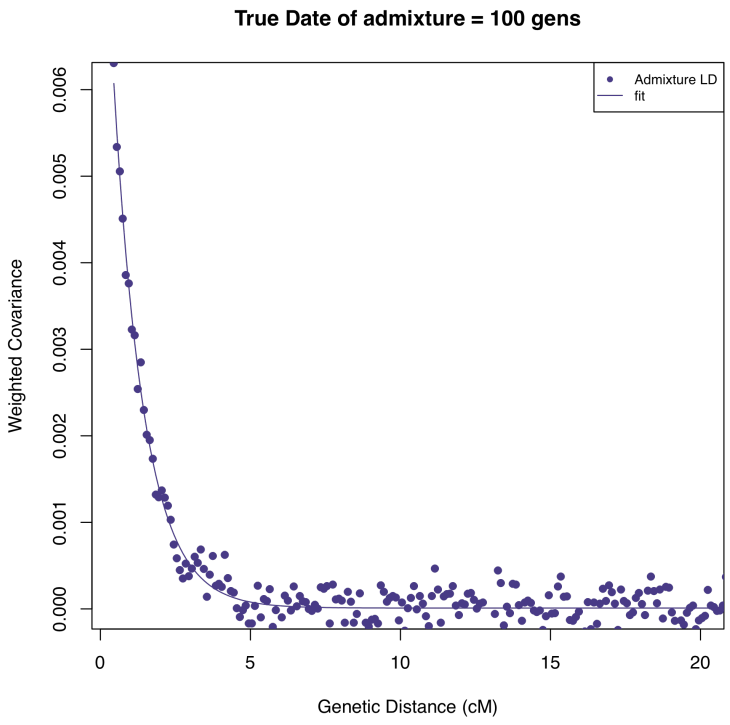

**Figure S6. IBD Sharing of Roma with host European populations.** We computed average pairwise IBD sharing between Roma from each geographical region and Europeans from that region (non-Roma European individuals from the countries in which the Roma were sampled).

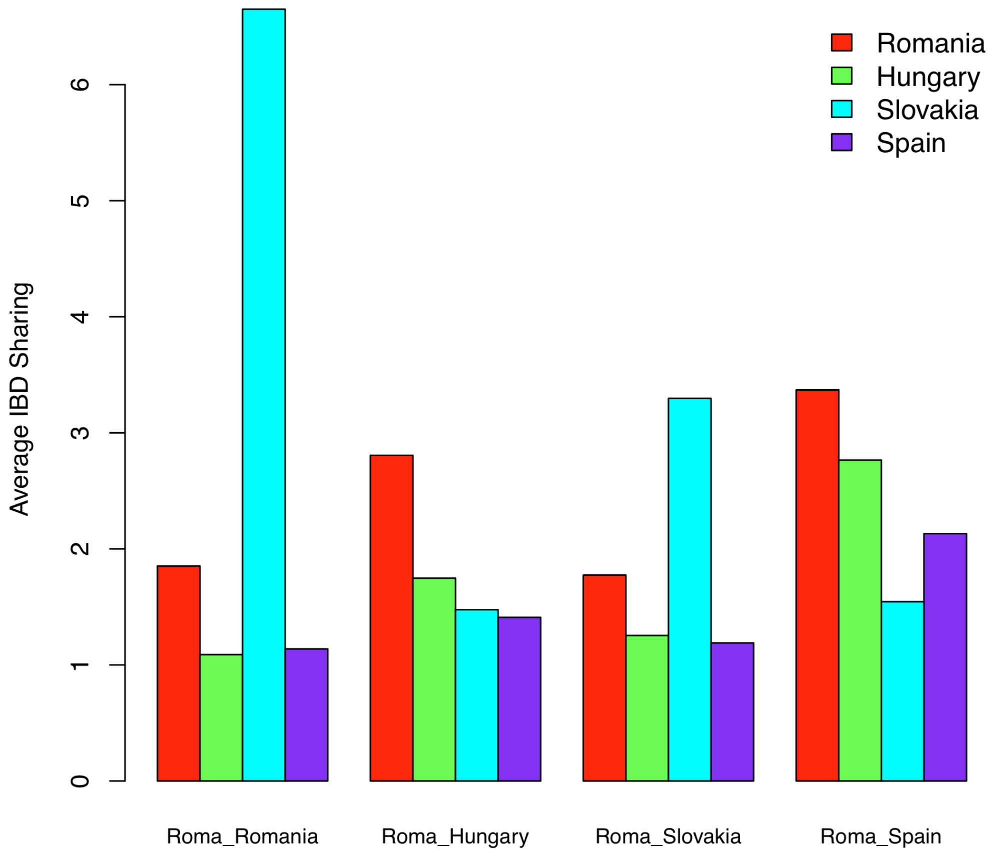

**Figure S7. Bootstrap analysis to compute error in IBD statistics.** We performed bootstrap analysis where we randomly sample up to 30 individuals from each of the 8 Indian groups and compute the IBD sharing statistics between Roma and the Indian groups. We performed a total of 100 runs and obtained the mean and standard error of the IBD statistic (vertical bars shown below). For Indian groups which had < 30 samples (such as Northeast, Southwest, East and Andamanese), all samples were included in each run and so no standard errors are shown.

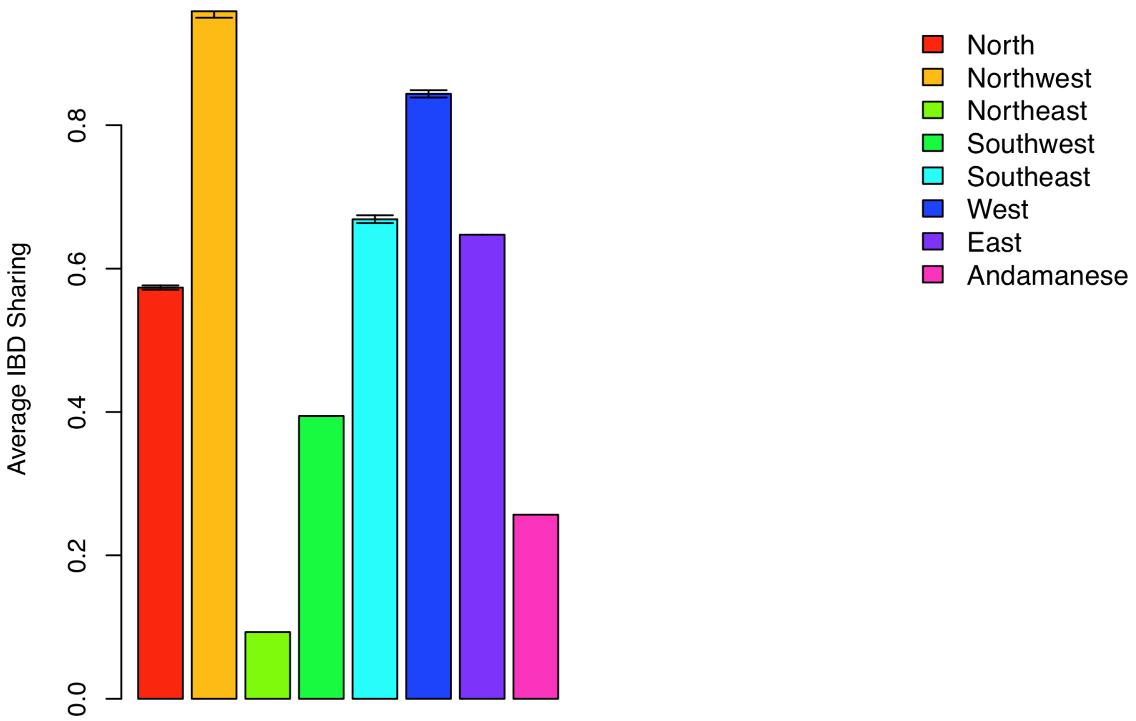

**Table S1. Average frequency differentiation ($F_{st}$) for Roma and HapMap populations**

| | CEU | YRI | CHB | JPT | ASW | CHD | GIH | LWK | MEX | MKK | TSI | Roma |
|---|---|---|---|---|---|---|---|---|---|---|---|---|
| **CEU** | 0 | 0.14 | 0.102 | 0.104 | 0.088 | 0.103 | 0.033 | 0.13 | 0.036 | 0.093 | 0.003 | 0.016 |
| **YRI** | 0.14 | 0 | 0.169 | 0.17 | 0.008 | 0.169 | 0.129 | 0.007 | 0.134 | 0.025 | 0.136 | 0.135 |
| **CHB** | 0.102 | 0.169 | 0 | 0.007 | 0.127 | 0.001 | 0.071 | 0.159 | 0.064 | 0.131 | 0.102 | 0.092 |
| **JPT** | 0.104 | 0.17 | 0.007 | 0 | 0.129 | 0.008 | 0.072 | 0.161 | 0.065 | 0.133 | 0.104 | 0.094 |
| **ASW** | 0.088 | 0.008 | 0.127 | 0.129 | 0 | 0.128 | 0.083 | 0.009 | 0.088 | 0.013 | 0.086 | 0.087 |
| **CHD** | 0.103 | 0.169 | 0.001 | 0.008 | 0.128 | 0 | 0.071 | 0.16 | 0.066 | 0.132 | 0.103 | 0.093 |
| **GIH** | 0.033 | 0.129 | 0.071 | 0.072 | 0.083 | 0.071 | 0 | 0.119 | 0.038 | 0.086 | 0.032 | 0.026 |
| **LWK** | 0.13 | 0.007 | 0.159 | 0.161 | 0.009 | 0.16 | 0.119 | 0 | 0.125 | 0.015 | 0.126 | 0.125 |
| **MEX** | 0.036 | 0.134 | 0.064 | 0.065 | 0.088 | 0.066 | 0.038 | 0.125 | 0 | 0.093 | 0.037 | 0.04 |
| **MKK** | 0.093 | 0.025 | 0.131 | 0.133 | 0.013 | 0.132 | 0.086 | 0.015 | 0.093 | 0 | 0.088 | 0.089 |
| **TSI** | 0.003 | 0.136 | 0.102 | 0.104 | 0.086 | 0.103 | 0.032 | 0.126 | 0.037 | 0.088 | 0 | 0.015 |
| **Roma** | 0.016 | 0.135 | 0.092 | 0.094 | 0.087 | 0.093 | 0.026 | 0.125 | 0.04 | 0.089 | 0.015 | 0 |

## Table S2. Formal tests of admixture

| Population (*X*) | Sam-ples | Region | *Z*-score for *4 Population test* ($P_{CEU}$-$P_{YRI}$) × ($P_{Onge}$- $P_X$) | ($P_{YRI}$-$P_{Onge}$) × ($P_{CEU}$-$P_X$) | ($P_x$-$P_{YRI}$) × ($P_{CEU}$-$P_{Onge}$) | Estimated West Eurasian Ancestry % |
|---|---|---|---|---|---|---|
| Roma | 18 | Hungary | -33 | 4.8 | -29.3 | 78.3 ± 1.9% |
| Roma* | 3 | Slovakia | -26.6 | 3.5 | -22.8 | 71.5 ± 3.1% |
| Roma** | 1 | Romania | -20.2 | 0.7 | -19.2 | 79.4 ± 4.7% |
| Roma | 2 | Spain | -25.3 | 0.9 | -24 | 75.6 ± 4.0% |
| Roma | 24 | Combined | -33 | 4.8 | -29.5 | 77.5 ± 1.8% |

*NOTE:* * indicates that some samples from the group appear to have recent European gene flow. These samples were excluded from the analysis (the number of * indicates the number of samples excluded). Ancestry proportions were estimates based on $f_4$ *Ratio Estimation* using Yoruba, Adygei, Europeans (CEU) and Onge as the reference populations.

## Table S3. Simulations for estimating dates of admixture events: Founder events post admixture model

| True date of admixture | True date of founder event ($x$) | Date based on original *ROLLOFF* statistic (a) | Date based on modified *ROLLOFF* statistic (b) | Date based on modified *ROLLOFF* statistic (c) |
|---|---|---|---|---|
| 30 | N/A | 31.3 | 32.0 | 32.1 |
| 30 | 5 | 24.6 | 30.1 | 29.0 |
| 30 | 10 | 27.7 | 34.1 | 32.3 |
| 30 | 20 | 23.3 | 32.7 | 31.0 |
| 30 | 25 | 23.4 | 30.8 | 29.5 |
| | | | | |
| 100 | N/A | 94.1 | 96.8 | 97.0 |
| 100 | 10 | 93.9 | 106.1 | 102.9 |
| 100 | 20 | 87.1 | 102.7 | 97.3 |
| 100 | 40 | 75.3 | 95.6 | 92.2 |
| 100 | 60 | 83.9 | 106.3 | 102.8 |
| 100 | 100 | 81.6 | 101.1 | 99.0 |

Note: We simulated data from three populations Pop A (n = 20), Pop B (n = 20) and Pop C (n = 30) using MaCS coalescent simulator. Populations A and B diverged 1800 generations ago. The effective population size for all populations was set 12,500 at all times (except during the founder event). The mutation and recombination rates were set to $2 \times 10^{-8}$ and $1 \times 10^{-8}$ per base pair per generation. Pop C can be considered as an admixed population that has ancestry 60%/40% ancestry from A' and B' (admixture time (t) is set to 30/ 100 generations). Pop A' and A diverged 120 generations and B' and B diverged 200 generations ago. At generation $x$ (shown in table above), Pop C undergoes a severe founder event where the effective population size reduces to 5 individuals for one generation. When $x$ = N/A, there was no founder event. We performed *ROLLOFF* (using original and modified statistic) with Pop C as the target and Pop A and B as the reference populations. We performed 5 replicates for each parameter and report the average estimated date of mixture. The statistics used were -

(a) Original *ROLLOFF* Statistic: $A(d) = \frac{\sum_{|x-y|\approx d} z(x,y)w(x,y)}{\sqrt{\sum_{|x-y|\approx d} z(x,y)^2}\sqrt{\sum_{|x-y|\approx d} w(x,y)^2}}$; where $z(x,y)$ = correlation between $x$ and $y$.

(b) Modified Statistic: $R(d) = \frac{\sum_{|x-y|\approx d} z(x,y)w(x,y)}{\sum_{|x-y|\approx d} w(x,y)^2}$; where $z(x,y)$ = correlation between $x$ and $y$.

(c) Modified Statistic: $R(d) = \frac{\sum_{|x-y|\approx d} z(x,y)w(x,y)}{\sum_{|x-y|\approx d} w(x,y)^2}$; where $z(x,y)$ = ***covariance*** between $x$ and $y$.

**Table S4. Simulations for estimating dates of admixture events: Two gene flow model**

| Date of first wave of mixture ($\lambda_1$) | Date of second wave of mixture ($\lambda_2$) | Estimated date in generations (± standard error) |
|---|---|---|
| 120 | 20 | 36 ± 3 |
| 170 | 20 | 28 ± 2 |
| 220 | 20 | 23 ± 2 |
| 270 | 20 | 24 ± 2 |
| 320 | 20 | 25 ± 1 |
| 370 | 20 | 25 ± 1 |
| 420 | 20 | 22 ± 1 |
| | | |
| 130 | 30 | 46 ± 3 |
| 180 | 30 | 47 ± 3 |
| 230 | 30 | 41 ± 2 |
| 280 | 30 | 39 ± 2 |
| 330 | 30 | 39 ± 3 |
| 380 | 30 | 35 ± 2 |
| 430 | 30 | 32 ± 3 |

Note: We simulated 27 individuals using CEU and Han Chinese as the ancestral populations where we set the overall European ancestry proportion to be 80%. We then performed *ROLLOFF* analysis using the modified statistic with an independent dataset of Europeans (HGDP French) and East Asians (HapMap CHB) as reference populations.

## Table S5. Simulations for estimating dates of founder events

| Simulation scenario | True date of founder event | True date of admixture | Estimated date of founder event (in generations) |
|---|---|---|---|
| **Founder event only** | | | |
| | 10 | -- | 11.2 |
| | 20 | -- | 20.8 |
| | 40 | -- | 39.3 |
| | 60 | -- | 52.7 |
| | 80 | -- | 74.9 |
| | 100 | -- | 95.7 |
| | | | |
| **Founder event + Admixture** | | | |
| | 10 | 10 | 8.2 |
| | 10 | 20 | 8.4 |
| | 10 | 40 | 8.3 |
| | 10 | 60 | 9.2 |
| | 10 | 80 | 11.8 |
| | 10 | 100 | 9.9 |
| | 30 | 10 | 24.4 |
| | 30 | 20 | 29.9 |
| | 30 | 30 | 30.1 |
| | 30 | 40 | 26.5 |
| | 30 | 60 | 26.2 |
| | 30 | 80 | 27.9 |
| | 30 | 100 | 27.6 |
| | 100 | 10 | 50 |
| | 100 | 20 | 60.9 |
| | 100 | 40 | 67.4 |
| | 100 | 60 | 81.5 |
| | 100 | 80 | 113.3 |
| | 100 | 100 | 92.7 |
| | 100 | 150 | 85.3 |

Note: We simulated 20 individuals from Pop A and 25 individuals from Pop B using MaCS coalescent simulator. The two populations diverged 1800 generations ago. The effective population size for both populations was set 12,500 at all times (except during the founder event). The mutation and recombination rates were set to $2 \times 10^{-8}$ and $1 \times 10^{-8}$ per base pair per generation. During the founder event, the effective population size reduced to 5 individuals for one generation at the date specified in the table above. For each simulation we generated data for ~450,000 polymorphic sites. SNPs with minor allele frequencies of <1% were discarded.

***References***

1. Moorjani P, Patterson N, Hirschhorn JN, Keinan A, Hao L, et al. (2011) The History of African Gene Flow into Southern Europeans, Levantines, and Jews. PLoS Genetics 7: e1001373.
2. Hill W, Robertson A (1968) Linkage disequilibrium in finite populations. TAG Theoretical and Applied Genetics 38: 226-231.
3. Chen GK, Marjoram P, Wall JD (2009) Fast and flexible simulation of DNA sequence data. Genome Research 19: 136-142.
4. Reich D, Thangaraj K, Patterson N, Price A, Singh L (2009) Reconstructing Indian population history. Nature 461: 489-494.
